# Supplementary material for: The Cellular Homology of Digraphs
Source: arXiv:2402.05682 source file (2025-05-22)

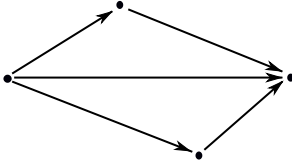

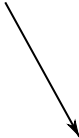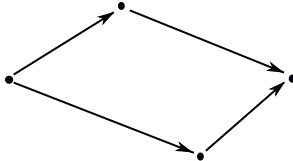

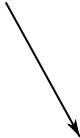

Supplement: Supplementary file 1 [file suppex.pdf]
